# Supplementary material for: Beyond Masked and Unmasked: Discrete Diffusion Models via Partial Masking
Source: arXiv:2505.18495 source file (2025-10-22)
Supplement: Supplementary file 1 [file nll.tex]

\begin{equation}
\label{eq:apx:nll}
\begin{aligned}
\E_{\vx\sim p}[-\log q(\vx)]&=\sum_{\vx\in\X} p(\vx)\log q(\vx)
\\&=\sum_{\vy\in \Y} p(f^{-1}(\vy))\log q(f^{-1}(\vy))=\E_{\vy\sim p\circ f^{-1}}[-\log q(f^{-1}(\vy))].
\end{aligned}
\end{equation}
