# Supplementary material for: Beyond Masked and Unmasked: Discrete Diffusion Models via Partial Masking
Source: arXiv:2505.18495 source file (2025-10-22)
Supplement: Supplementary file 3 [file gen_ppl.tex]

\begin{table}[t]
    
    \newcommand{\boldtoprule}{\toprule[0.9pt]}
    \newcommand{\boldbottomrule}{\bottomrule[0.9pt]}
    \centering
    \caption{A comparison of Gen PPL and Entropy evaluated under different number of sampling timesteps. MDM-Prime adopts the setup with $\ell=6$. }
    \small
    \begin{tabular}{ccccc}
        \boldtoprule
                            & Timesteps  & Gen PPL (LLaDA) ($\downarrow$) & Gen PPL (GPT-2) ($\downarrow$) & Entropy ($\uparrow$) \\
        \hline
        ARM & 1024 & 93.0 & 38.0 & 7.98 \\
        MDLM & 512 / 1024 / 2048 & 74.5 / 63.8 / 56.3 & 105.0 / 96.0 / 93.0 &  8.06 / 8.09 / 8.04 \\
        MDLM-Prime  &  512 / 1024 / 2048  & 77.0 / 49.8 / 40.5 & 93.0 / 90.0 / 84.5  &  7.70 / 7.67 / 7.65 \\
        \boldbottomrule
    \end{tabular}
    \label{tab:apx:gen_ppl}
\end{table}
